# Supplementary material for: Unified Perceptive Fall Safety for Humanoids
Source: arXiv:2602.16511 source file (2026-10-15)
Supplement: Supplementary file 1 [file rss_only_appendix.tex]

\documentclass[conference]{IEEEtran}
\usepackage{times}

\usepackage[numbers]{natbib}
\usepackage{multicol}
\usepackage[bookmarks=true]{hyperref}
\usepackage{graphicx}
\usepackage{graphics}
\usepackage{epsfig}
\usepackage{times}
\usepackage{subcaption}
\usepackage{amsmath}
\usepackage{amssymb}
\usepackage[table]{xcolor}
\usepackage{colortbl}
\usepackage{placeins}

\usepackage[ruled,linesnumbered, noend]{algorithm2e}
\usepackage{soul}
\usepackage{comment}
\usepackage{siunitx}

\usepackage{multirow}
\usepackage{wrapfig}
\usepackage{soul, color}
\usepackage{mathtools}
\usepackage{booktabs}
\usepackage{adjustbox}
\usepackage{caption}
\usepackage{lipsum}

\usepackage{xspace}

% If your appendix relies on these files, keep them:
% \input{figTeaser.tex} % harmless if it defines macros; remove if it inserts a figure
% \input{paper-template-latex/sim_table} % only if appendix needs it via direct call
% \input{paper-template-latex/real_tables} % only if appendix needs it via direct call

\begin{document}

% Top-of-page supplementary header (like your screenshot)
\twocolumn[{%
\begin{@twocolumnfalse}
\begin{center}
{\LARGE\bfseries VIGOR: Visual Goal-In-Context Inference for\\[0.6em]
Unified Humanoid Fall Safety}\\[0.8em]
{\Large Supplementary Material}
\end{center}
\end{@twocolumnfalse}
}]

% \appendix
\input{paper-template-latex/08_appendix}

\FloatBarrier

% optional: appendix-only references (uses same references.bib)
\bibliographystyle{plainnat}
\bibliography{references}

\end{document}
